# Supplementary material for: Subtyping on Nested Polymorphic Session Types
Source: arXiv:2103.15193 source file (2021-03-28)
Supplement: Supplementary file 1 [file appendix.tex]

\section{Appendix}
\label{sec:appendix}

\subsection{Properties of variance}

\begin{lemma}[Variance] The following properties hold.
\label{lem:properties_variance}
\begin{enumerate}
\item If $\vars\semi \Xi \vdash A \ofv \xi$ and $\xi' \leq \xi$ then $\vars\semi \Xi \vdash A \ofv \xi'$.
\item If $\vars\semi \Xi, \alpha \ofv \xi \vdash A \ofv \zeta$ and $\xi \leq \xi'$
  then $\vars\semi \Xi, \alpha \ofv \xi' \vdash A \ofv \zeta$.
\item If $\vars\semi \Xi \vdash A \ofv \xi$ and $\vars\semi \Xi, \alpha \ofv \xi \vdash C \ofv \zeta$
  then $\vars\semi \Xi \vdash C[A/\alpha] \ofv \zeta$.
\item If $\vars\semi \Xi \vdash \theta \ofv \Xi'$ and $\vars\semi\Xi' \vdash C \ofv \zeta$
  then $\vars\semi \Xi \vdash C[\theta] \ofv \zeta$. 
\item If $\vars\semi \Xi \vdash A \ofv \xi$ then $\vars\semi\Xi \mid \xi' \vdash A \ofv \xi \mid \xi'$.
\item If $\vars\semi \Xi \vdash V[\theta'] \ofv \xi$ and $V[\Xi'] = A' \in \Sigma_0$
  then $\vars\semi \Xi \vdash A'[\theta'] \ofv \xi$.
\item If $\vars\semi \Xi \vdash \theta \ofv \Xi'$ and 
	$\vars\semi \Xi' \vdash \theta_V \ofv \Xi_V$, then 
	$\vars\semi \Xi \vdash \theta_V[\theta] \ofv \Xi_V$.
\end{enumerate}
\end{lemma}
\begin{proof}\
	\begin{enumerate}
		\item Proof by induction, using transitivity of $\leq$ and monotonicity of nesting.
		\item Proof by induction, using transitivity of $\leq$.
		\item Proof by induction, using (1).
		\item Proof by induction, using (3).
		\item Proof by induction, using associativity of nesting.
		\item Proof by inversion, using (5), (4), and $\cov \mid \xi = \xi$.
		\item Proof by induction, using (4).
	\end{enumerate}
	\vspace*{-1em}
\end{proof}

%\begin{lemma}[Substitutions composition] If $\vars\semi \Xi \vdash V[\theta_V] \ofv \xi$ and
%	$\vars'\semi \Xi' \vdash \theta \ofv \Xi$ and $V[\Xi_V]=A \in \Sg$, then:
%	\begin{enumerate}
%	\setcounter{enumi}{7}
%	\item $\vars'\semi \Xi' \vdash V[\theta_V][\theta] \ofv \xi$.
%	\item $\vars'\semi \Xi' \vdash V[\theta_V[\theta]] \ofv \xi$.
%	\item $A[\theta_V][\theta] =  A[\theta_V[\theta]]$.
%	\item $\unfold{V[\theta_V][\theta]} =  \unfold{V[\theta_V[\theta]]}$.
%	\end{enumerate}
%\end{lemma}
%\begin{proof}\
%	\begin{enumerate}
%	\setcounter{enumi}{7}
%		\item Immediate from (4).
%		\item Since $\vars\semi \Xi \vdash V[\theta_V] \ofv \xi$, we have
%		$\vars\semi \Xi \vdash \theta_V \ofv \Xi_V\mid \xi$. \\
%		By (7), we know that
%		$\vars'\semi \Xi' \vdash \theta_V[\theta] \ofv \Xi_V\mid \xi$.\\
%		Applying the last rule for valid types, we get 
%		$\vars'\semi \Xi' \vdash V[\theta_V[\theta]] \ofv \xi$.
%		\item Proof by induction on the structure of $A$, knowing that 
%		$\cdot\semi \Xi_V \vdash A \ofv \cov$ and using (5) and (4).
%		\item Immediate from (10).
%	\end{enumerate}
%\end{proof}

\begin{lemma}[Continuation types]
	Given a type $V[\theta]$ s.t. $\vars\semi \Xi \vdash V[\theta] \ofv \delta$
		and $V[\Xi_V]=A \in \Sg_0$, if $V_0[\theta_A]$ is a  continuation type 
		occurring in a position of variance $\xi$ on $A$ and
		s.t. $V_0[\Xi_0]=B \in \Sg_0$, then
		$\vars'\semi \Xi \vdash V_0[\theta_A[\theta]] \ofv \xi\mid \delta$.
\end{lemma}
%\begin{proof}[Proof 1]
%	By induction on the structure of $A$.
%\end{proof}
\begin{proof}
	Since $\vars\semi \Xi \vdash V[\theta] \ofv \delta$, we know that 
	\begin{equation}
		\label{eq:theta_var_appdx}
		\vars\semi \Xi \vdash \theta \ofv \Xi_V\mid \delta.
	\end{equation}
	On the other hand, since $\cdot\semi \Xi_V \vdash A \ofv \cov$
	and $V_0[\theta_A]$ occurs at position of variance $\xi$, we have
	$\vars'\semi \Xi_V \vdash V_0[\theta_A] \ofv \xi$. Hence, 
	we know that $\vars'\semi \Xi_V \vdash \theta_A \ofv \Xi_0\mid \xi$.
	Using (5) we also have 
	\begin{equation}
		\label{eq:thetaA_var_appdx}
		\vars'\semi \Xi_V\mid \delta \vdash \theta_A \ofv (\Xi_0\mid \xi) \mid\delta
	\end{equation}
	By equations~\eqref{eq:theta_var_appdx},~\eqref{eq:thetaA_var_appdx}, and Lemma~\ref{lem:properties_variance} (7), we have 
	$\vars\semi \Xi \vdash \theta_A[\theta] \ofv (\Xi_0\mid \xi) \mid\delta.$
	Using associativity of nesting and the rule for valid type names, we get
	$\vars'\semi \Xi \vdash V_0[\theta_A[\theta]] \ofv \xi\mid \delta$.
\end{proof}

%\begin{lemma}[Variance and subtyping] Given $A$ and $B$ such that 
%$\vars\semi \Xi \vdash A \ofv \xi$ and $\vars\semi \Xi \vdash B \ofv \xi$,
%the following properties hold.
%\begin{enumerate}
%\item If $\vars \semi \G \vdash A \leq B \ofv \xi$ and $\xi' \leq \xi$ then $\vars \semi \G \vdash A \leq B \ofv \xi'$.
%\item If $\vars \semi \G \vdash A \leq B \ofv \xi$ then $\vars \semi \G \vdash B \leq A \ofv \lnot\xi$.
%\item If $\vars \semi \G \vdash \theta \leq \theta' \ofv \Xi'$ and $\vars\semi\Xi' \vdash A \ofv \xi$
%  then $\vars \semi \G \vdash A[\theta] \leq A[\theta'] \ofv \xi$
%\item If $\vars \semi \G \vdash \theta \leq \theta' \ofv \Xi'$ and $\vars\semi\Xi' \vdash \theta_V \ofv \Xi_V$
%  then $\vars \semi \G \vdash \theta_V[\theta] \leq \theta_V[\theta'] \ofv \Xi_V$
%\end{enumerate}	
%\end{lemma}
%
%\begin{proof}
%	\textcolor{blue}{am: todo}
%\end{proof}

\subsection{Soundness of the subtyping algorithm}

In this subsection, we present the proof of the subtyping algorithm.
Recall that our soundness result (Theorem~\ref{thm:soundness}) states that:\smallskip

\begin{center}
	\begin{minipage}{0.9\textwidth}
	 For valid types $A$ and $B$ s.t.
  $\vars \semi \cdot \vdash A \ofv \delta$
  and $\vars \semi \cdot \vdash B \ofv \delta$, if
  the subtyping algorithm proves
  $\vars \semi \cdot \vdash A \leq B \ofv \delta$,
  then $\forall \vars.\, A \leq B \ofv \delta$.
	\end{minipage}
\end{center}

\begin{proof}[Proof of Theorem~\ref{thm:soundness}]:
  Given $A_0, B_0$ s.t. 
  $\vars_0 \semi \cdot \vdash A_0 \ofv \delta$
  and $\vars_0 \semi \cdot \vdash B_0 \ofv \delta$ and a 
  derivation $\mathcal{D}_0$ of $\vars_0 \semi \cdot
  \vdash A_0 \leq B_0 \ofv \delta$, construct the set
  of closures $\mathcal{S}(\mathcal{D}_0)$. Define a relation
  $\rel_0$ such that
%  \begin{eqnarray*}
%    \rel_0 & = & \{(A_0[\sigma], B_0[\sigma]) \mid \clo{\vars}{A_0 \leq B_0 \ofv \cov}
%    \in \mathcal{S}, \; \mbox{and $\sigma$ over $\vars$}\}\\
%    & \cup & \{(B_0[\sigma], A_0[\sigma]) \mid \clo{\vars}{A_0 \leq B_0 \ofv \conv}
%    \in \mathcal{S}, \; \mbox{and $\sigma$ over $\vars$}\}\\
%    & \cup & \{(A_0[\sigma], B_0[\sigma]), (B_0[\sigma], A_0[\sigma])
%    \mid \clo{\vars}{A_0 \leq B_0 \ofv \biv}
%    \in \mathcal{S}, \; \mbox{and $\sigma$ over $\vars$}\}
%  \end{eqnarray*}
  \begin{eqnarray*}
    \rel_0 & = & \{(A[\sigma], B[\sigma]) \mid \clo{\vars}{A \leq B \ofv \cov}
    \in \mathcal{S}(\mathcal{D}_0) \text{ and $\sigma$ closed substitution  over $\vars$}\}\\
    & \cup & \{(B[\sigma], A[\sigma]) \mid \clo{\vars}{A \leq B \ofv \conv}
    \in \mathcal{S}(\mathcal{D}_0) \text{ and $\sigma$ closed substitution over $\vars$}\}\\
    & \cup & \{(A[\sigma], B[\sigma]), (B[\sigma], A[\sigma])
    \mid \clo{\vars}{A \leq B \ofv \biv}
    \in \mathcal{S}(\mathcal{D}_0), \text{ $\sigma$ closed substitution over $\vars$}\}
    %, \; \mbox{and $\sigma$ over $\vars$}
  \end{eqnarray*} 
  Recall the variance-based relation defined in Definition~\ref{def:variance_based_rel}
  and note that $\clo{\vars}{A \leq B \ofv \delta}
  \in \mathcal{S}(\mathcal{D}_0)$ iff $(A[\sigma],B[\sigma])\in\rel_0^\delta$,
  for any closed substitution $\sigma$ over $\vars$.
  Then, let $\rel$ be the reflexive and transitive closure of $ \bigcup_{i\geq 0} \rel_i$ 
  where, for $i\geq 1$:
%  \[
%    \rel_1 = \{(V[\theta_A], V[\theta_B]) \mid V[\Xi] = C \in \Sg \text{ and }
%    (\alpha \ofv \delta) \in \Xi \implies (A/\alpha) \in \theta_A \text{ and }
%    (B/\alpha) \in \theta_B \; \forall (A,B) \in R_0^{\delta} \}
%  \]
	\[
	\rel_i = \{(V[\theta_1], V[\theta_2]) \mid V[\Xi] = C \in \Sg \text{ and }
	(\alpha \ofv \xi) \in \Xi \Rightarrow
    (A/\alpha) \in \theta_1 \text{ and }
    (B/\alpha) \in \theta_2 \; \forall (A,B) \in R_{i-1}^{\xi}\}
    \]
%
  %Consider $\rel$ to be the \emph{reflexive transitive closure} of $\rel_0 \cup \rel_1$.
  We now prove that $\rel$ is a type simulation. Then, our theorem follows because
%  (i) 
	$\vars_0 \semi \cdot \vdash A_0 \leq B_0 \ofv \delta$ implies  
%	$\implies \vars \semi \cdot
%   \vdash A_0 \ofv \delta$ and $\vars \semi \cdot \vdash B_0 \ofv \delta$,
%  (ii) 
  $\clo{\vars_0}{A_0 \leq B_0 \ofv \delta} \in \mathcal{S}(\mathcal{D}_0)$.
  Then, for any closed substitution $\sigma$ over $\vars_0$, we have
  $(A_0[\sigma], B_0[\sigma]) \in \rel^\delta$, complying with 
  Definition~\ref{def:subtp}.

  Note that extending a relation by its reflexive and transitive closure
  preserves the simulation properties.
  To prove that $\rel$ is a type simulation, we
  consider $(A[\sigma], B[\sigma]) \in \rel^\delta$ where
  $\clo{\vars}{A \leq B \ofv \delta} \in \mathcal{S}(\mathcal{D}_0)$ and
  $\sigma$ is a substitution over $\vars$. We case analyze on the rule in the
  derivation which added the above closure to $\rel$.

  Consider the case where $\ichoiceop_\conv$ rule is applied
  to add $(B[\sigma], A[\sigma]) \in \rel$, i.e.,
  $(A[\sigma], B[\sigma]) \in \rel^\conv$.
  The rule dictates that $A = \ichoice{\ell : A_\ell}_{\ell \in L}$
  and $B = \ichoice{m : B_m}_{m \in M}$. Since
  $\clo{\vars}{A \leq B \ofv \conv} \in \mathcal{S}(\mathcal{D}_0)$,
  by Lemma~\ref{lem:closure}, we obtain that $L \supseteq M$ and
  $\clo{\vars}{A_m \leq B_m \ofv \conv} \in \mathcal{S}(\mathcal{D}_0)$ for all
  $m \in M$. By the definition of $\rel$, we get that
  $(B_m[\sigma], A_m[\sigma]) \in \rel$. Also,
  $A[\sigma] = \ichoice{\ell : A_\ell[\sigma]}_{\ell \in L}$ and similarly,
  $B[\sigma] = \ichoice{m : B_m[\sigma]}_{m \in M}$.  Hence, $\rel$ satisfies the
  closure condition (case 1) from Definition~\ref{def:subtp_rel}.
  The cases for $\ichoiceop_\cov$ and $\ichoiceop_\biv$ are analogous.

  Consider the case where $\echoiceop_\conv$ rule is applied
  to add $(B[\sigma], A[\sigma]) \in \rel$, i.e.,
  $(A[\sigma], B[\sigma]) \in \rel^\conv$.
  The rule dictates that $A = \echoice{\ell : A_\ell}_{\ell \in L}$
  and $B = \echoice{m : B_m}_{m \in M}$. Since
  $\clo{\vars}{A \leq B \ofv \conv} \in \mathcal{S}(\mathcal{D}_0)$,
  by Lemma~\ref{lem:closure}, we obtain that $L \subseteq M$ and
  $\clo{\vars}{A_\ell \leq B_\ell \ofv \conv} \in \mathcal{S}(\mathcal{D}_0)$ for all
  $\ell \in L$. By the definition of $\rel$, we get that
  $(B_\ell[\sigma], A_\ell[\sigma]) \in \rel$. Also,
  $A[\sigma] = \echoice{\ell : A_\ell[\sigma]}_{\ell \in L}$ and similarly,
  $B[\sigma] = \echoice{m : B_m[\sigma]}_{m \in M}$.  Hence, $\rel$ satisfies the
  closure condition (case 2) from Definition~\ref{def:subtp_rel}.
  The cases for $\echoiceop_\cov$ and $\echoiceop_\biv$ are analogous.

  If the applied rule is $\lolli$, then $A = A_1 \lolli A_2$
  and $B = B_1 \lolli B_2$. Lemma~\ref{lem:closure} implies
  that $\clo{\vars}{A_1 \leq B_1 \ofv \neg \delta} \in \mathcal{S}(\mathcal{D}_0)$
  and $\clo{\vars}{A_2 \leq B_2 \ofv \delta} \in \mathcal{S}(\mathcal{D}_0)$.
  We get that $(A_1[\sigma],B_1[\sigma]) \in \rel^{\neg\delta}$
  and $(A_2[\sigma], B_2[\sigma]) \in \rel^\delta$.
  From which we conclude that $(B_1[\sigma], A_1[\sigma]) \in \rel^\delta$ 
  and $\rel$ satisfies the
  closure condition (case 3) from Definition~\ref{def:subtp_rel}.

  The case of $\tensor$ is analogous to $\lolli$. The case for $\one$
  is trivial.

  If the applied rule is $\exists^z$, then $A = \texists{x} A'$
  and $B = \texists{y} B'$ and $(A[\sigma], B[\sigma]) \in \rel^\delta$.
  Lemma~\ref{lem:closure} implies
  that $\clo{\vars,z}{A'[z/x] \leq B'[z/y] \ofv \delta} \in
  \mathcal{S}(\mathcal{D}_0)$.
  Thus, the definition of $\rel$ ensures that $(A'[z/x][\sigma'], B'[z/y][\sigma']) \in \rel^\delta$
  for any $\sigma'$ closed substitution over $\vars, z$.
  Also, $A[\sigma] = \texists{x} A'[\sigma]$ and
  $B[\sigma] = \texists{y} B'[\sigma]$.
  To satisfy the closure condition, we need to prove that
  $(A'[\sigma][C/x], B'[\sigma][C/y]) \in \rel^\delta$ for any $C \in \mi{Type}$.
  Setting $\sigma' = \sigma, C/z$, we get that
  $A'[z/x][\sigma'] = A'[z/x][\sigma,C/z] = A'[\sigma][C/x]$.
  Similarly, $B'[z/x][\sigma'] = B'[\sigma][C/y]$.
  Combining, we get that $(A'[\sigma][C/x], B'[\sigma][C/y]) \in \rel^\delta$.

  The case for $\forall^z$ is analogous to $\exists^z$.

  If the applied rule is $\m{var}$, then $A = x$ and $B = x$.
  In this case, the relation $\rel$ contains any $(C, C)$ for
  a closed session type $C$ s.t. $\sigma(x) = C$.
  To prove $\rel$ is a type simulation, we need to subcase on the form of $C$.
  For instance, if $C$ is of the form $\ichoice{\ell : C_\ell}_{\ell \in L}$,
  then we need to prove that $(C_\ell, C_\ell) \in \rel$ for all $\ell \in L$.
  But since $C_\ell$ is a closed session type, the reflexivity condition of $\rel$
  implies that it contains $(C_\ell, C_\ell)$.
  The remaining subcases are analogous.
  
  If the applied rule is $\nonv$, nothing is added to $\rel$.
  Thus, the result holds vacuously. (Also, recall that 
  $\rel^\nonv$ relates any two types, by definition.)

  Consider the case where $\m{expd}$ rule is applied. In this case,
  $A = V_1[\theta_1]$ and $B = V_2[\theta_2]$ and $(A[\sigma], B[\sigma]) \in \rel^\delta$.
  Suppose the definitions are $V_1[\Xi_1] = C_1$ and $V_2[\Xi_2] = C_2$.
  Note that $\unfold{A} = C_1[\theta_1]$ and
  $\unfold{B} = C_2[\theta_2]$. From Lemma~\ref{lem:closure},
  we conclude that $\clo{\vars}{C_1[\theta_1] \leq
  C_2[\theta_2] \ofv \delta} \in \SDO$.
  Since the next applied rule has to be a structural rule,
  we can use Lemma~\ref{lem:closure} again to obtain the closure conditions
  of a type simulation.

  The most crucial case is when the applied rule is $\m{def}$ as we attempt to
  close off the loop here. 
  In this case,
  $	\clo{\vars}{A \leq B \ofv \delta} \in \SDO$.
  Here,
  $A = V_1[\theta_1]$ and 
  $B = U_1[\theta_2]$,
  where the type definitions are
  	$V_1[\Xi_1] = C$ and 
  	$U_1[\Xi_2] = D$.
  And we also have $\clo{\vars'}{V_1[\theta_1'] \leq U_1[\theta_2']\ofv \delta} \in \SD$.
  The types $\unfold{A}$ and $\unfold{B}$ are structural. 
%  So, we reduce our analysis to
%  the structural cases. Consider the representative case where
%  $C=\ichoice{\ell : T_\ell}_{\ell \in L}$.
%  In this case, $D=\ichoice{m : U_m}_{m \in M}$ with $L \subseteq M$.
  Due to the internal renaming, 
  the continuation types for $C$ and $D$ are type names, 
  say 
  $V_2[\theta_{A}]$ and
  $U_2[\theta_{B}]$, respect., occurring in a position of variance $\xi$.
  Recalling that $(A[\sigma], B[\sigma]) \in \rel^\delta$,
%  where the type definitions 
%  $V_{C,\ell}[\Xi_1'] = E$ and 
%  $V_{D,m}[\Xi_2'] = F$ belong to $\Sigma$, for all $\ell$ and $m$.
  we want to prove that:
  \begin{equation}
  \label{eq:want_to_conclude_appdx}
  	(V_{2}[\theta_{A}[\theta_1]][\sigma], U_{2}[\theta_{B}[\theta_2]][\sigma])\in \rel^{\delta | \xi}.
  \end{equation}
  From Lemma~\ref{lem:closure}, we know that 
  exists a substitution $\sigma' : \vars' \to \mathcal{T}(\vars)$ s.t.
  $\clo{\vars}{V_1[\theta_1] \leq V_1[\theta_1'[\sigma']] \ofv \delta},
  	\clo{\vars}{U_1[\theta_2'[\sigma']] \leq U_1[\theta_2] \ofv \delta} \in \SDO$.
  Hence, we have
  \begin{equation}
  \label{eq:var_renaming_appdx}
  	(V_1[\theta_1][\sigma], V_1[\theta_1'[\sigma']][\sigma]),
  	(U_1[\theta_2'[\sigma']][\sigma], U_1[\theta_2][\sigma])\in \rel^\delta.
  \end{equation}
%  Due to~\eqref{eq:original_types}, we also have
%  \begin{equation}
%  \label{eq:renamed_original_types}
%  	(V_1[\theta_1][\sigma'[\sigma]], V_2[\theta_2][\sigma'[\sigma]])\in \rel.
%  \end{equation}
  Since $\theta_1$ and $\theta_2$  are a nesting of type names,
%  have type expressions defined over variables in $\vars$, 
  we can rewrite~\eqref{eq:var_renaming_appdx} as:
  \begin{equation}
  \label{eq:var_renaming2_appdx}
  	(V_1 [\theta_1[\sigma]], V_1 [\theta_1'[\sigma'[\sigma]]]),
  	(U_1 [\theta_2'[\sigma'[\sigma]]],U_1 [\theta_2[\sigma]])\in \rel^\delta.
  \end{equation}
  The application of successive simulation steps on each type, eventually 
  reaches the type variables occurring in $C$ and $D$. As we observed before, 
  type variables not occurring in $C$ or $D$ are assigned variance $\nonv$, which
  is the degenerate case of our variance-based relations
  in Definition~\ref{def:variance_based_rel}.
  Hence, in any of these cases, 
  by applying successive simulation steps over~\eqref{eq:var_renaming_appdx}, we get:
  \begin{equation}
  \label{eq:thetas_in_rel_appdx}
  \begin{array}{ll}
  	(A_1[\sigma], A_1'[\sigma'[\sigma]])\in \rel^{\delta\mid \xi_1}
  	\text{ for all $A_1/\alpha\in\theta_1$ and
  $A_1'/\alpha\in\theta_1'$ and $\alpha\ofv\xi_1\in \Xi_1$}\\
   (A_2'[\sigma'[\sigma]], A_2[\sigma])\in \rel^{\delta\mid \xi_2}
   \text{ for all $A_2'/\beta\in \theta_2'$
  and $A_2/\beta\in \theta_2$ and $\beta\ofv\xi_2\in\Xi_2$}
  \end{array}
  \end{equation}
  The internal renaming ensures that
  $\theta_{A}$ and $\theta_{B}$ are a nesting of type names. Hence,
  from~\eqref{eq:thetas_in_rel_appdx} and definition of $\mathcal{R}_i$, we conclude that
  \begin{equation}
  \label{eq:bisim_step_appdx}
  	(V_{2}[\theta_{A}[\theta_1[\sigma]]], V_{2}[\theta_{A}[\theta_1'[\sigma'[\sigma]]]]),
  	(U_{2} [\theta_{B}[\theta_2'[\sigma'[\sigma]]]], U_{2} [\theta_{B}[\theta_2[\sigma]]])\in 
  	\rel_i^{\delta\mid\xi},
  	\text{ for some $i \geq 1$.}
  \end{equation}
  Since we also have 
  $\clo{\vars'}{V_1[\theta_1'] \leq U_1[\theta_2']\ofv \delta} \in \SD$
  (see Lemma~\ref{lem:closure}), it follows that
  \begin{equation}
  \label{eq:with_theta'_appdx}
  	(V_1[\theta_1'][\sigma'[\sigma]], U_1[\theta_2'][\sigma'[\sigma]])\in \rel^{\delta}.
  \end{equation}
  Proceeding to the continuation types $V_2[\theta_{A}]$ and
  $U_2[\theta_{B}]$ (occurring at variance $\xi$) and using~\eqref{eq:bisim_step_appdx}
  and transitivity,
  we conclude~\eqref{eq:want_to_conclude_appdx}, as we wanted.
%  \textcolor{red}{To conclude, we need to ensure that 
%  $(V_1[\theta_1'][\sigma'[\sigma]], V_2[\theta_2'][\sigma'[\sigma]])\in \rel$
%  and apply transitivity. Can we ensure this from~\eqref{eq:original_types}? 
%  We know that 
%  $(V_1[\theta_1][\sigma''], V_2[\theta_2][\sigma''])\in \rel,$
%  but $\theta_i\neq\theta_i'$.}

  The last two cases concern reflexivity, one that comes directly from
  the closure obtained from applying the $\m{refl}$ rule, and the other
  comes from the relation $\rel_i$.
  Let us first consider the case where closure $\clo{\vars}{V[\theta_1]
  \leq V[\theta_2] \ofv \delta} \in \SDO$, i.e., 
  	$(V[\theta_1][\sigma], V[\theta_2][\sigma])\in \rel^\delta$.
  Assume that $V[\Xi_V] = C \in \Sg$.
  Lemma~\ref{lem:closure} ensures that 
  	$\clo{\vars}{A \leq B \ofv \xi\mid\delta} \in \SDO$,
  	for all $A/\alpha \in \theta_1$ and $B/\alpha \in \theta_2$
  and $\alpha \ofv \xi \in \Xi_V$.
%  Validity of types ensures that
%  \begin{equation}
%  	\label{eq:thetas}
%  	\cdot \semi \Xi_V \vdash C \ofv \cov \text{ and }
%  	\vars \semi \Xi \vdash \theta_1 \ofv \Xi_V \mid \delta \text{ and }
%  	\vars \semi \Xi \vdash \theta_2 \ofv \Xi_V \mid \delta.
%  \end{equation}
  By definition of $\rel_0$, 
  we thus have
  \begin{equation}
  	\label{eq:arguments_in_R0_appdx}
  	(A[\sigma],B[\sigma])\in \rel_0^{\xi\mid \delta},
  	\text{ for each $A/\alpha \in \theta_1$ and $B/\alpha \in \theta_2$
  and $\alpha \ofv \xi \in \Xi_V$.}
  \end{equation} 
  We proceed with a continuation of $C$.
  Let $V_0[\theta_0]$ denote a continuation type occurring in a position 
  of variance $\eta$ on $C$, with definition $V_0[\Xi_0] = D$. 
  We can easily show (by case analysis on $C$) 
  that $\Xi_0\mid \eta \subseteq \Xi_V$.
%  Recalling~\eqref{eq:first_pair},
%  notice that want to conclude that 
%  $(V_\ell[\theta_1][\sigma],V_\ell[\theta_2][\sigma])\in \rel^\delta$.
%  By~\eqref{eq:thetas} and since $\Xi_\ell \subseteq \Xi$, we have 
%  \textcolor{blue}{$\vars \semi \cdot \vdash \theta_i \ofv (\Xi_\ell \mid \delta)$},
%  for $i = 1,2$. Hence, we get $\vars \semi \cdot \vdash V_\ell[\theta_i] \ofv \delta$.
  To conclude, recall that
  the intermediate renaming ensures that $\theta_0$ is itself a nesting
  of type names $V_1\cdots V_k$, for $k\geq 1$.
  Using~\eqref{eq:arguments_in_R0_appdx} and the definition of $\rel_{k+1}$,
  we have
  $(V_0[\theta_0[\theta_1[\sigma]]], V_0[\theta_0[\theta_2[\sigma]]])\in \rel^{\delta\mid \eta}$,
  as we wanted.
%  If $V_\ell[\Xi_\ell] = C_\ell$, validity of $C$ proves that
%  we get that $\vars \semi \Xi \vdash V_\ell[\theta_i] \ofv \cov$
%  implying \textcolor{red}{$\vars \semi \Xi \vdash \theta_i \ofv (\Xi_\ell \mid \cov)$}.
%  To prove $\rel$ is a simulation, we need to prove
%  $(V_\ell[\theta_1[\sigma]], V_\ell[\theta_2[\sigma]])
%  \in \rel$. Note however the internal renaming condition ensures that
%  $B_\ell = V_B \indv{\alpha}$ for some (possibly internal) type name $V_B$.
%  But then the definition of $\rel_1$ coupled with the consequence of
%  Lemma~\ref{lem:closure} ensures that $(V_B \indv{A_1[\sigma]}, V_B \indv{A_2[\sigma]})
%  \in \rel$, satisfying the closure condition.
  %The other structural subcases are analogous.
  In the subcase where $C = \alpha$ for $\alpha\ofv \xi \in\Xi$,
  the validity of $\Sg_0$ ensures that $\xi = \cov$.
  In this particular case, we have $V [\theta_1] = A$ and
  $V [\theta_2] = B$ and $\theta_1 = A/\alpha$ and $\theta_2 = B/\alpha$.
  From~\eqref{eq:arguments_in_R0_appdx}, we conclude that 
  $(A[\sigma], B[\sigma]) \in \rel_0^{\cov\mid\delta}$ and so
  $(A[\sigma], B[\sigma]) \in \rel^{\delta}$.
  Note that $\unfold{V [\theta_1][\sigma]} = A[\sigma]$.
  The next applied rule has to be a structural rule, so
  we can use Lemma~\ref{lem:closure} again to obtain the closure conditions
  of a type simulation.
  
  A similar argument covers the latter case where $(V [\theta_1][\sigma], V [\theta_2][\sigma])
  \in \rel$ due to $\rel_i$.

  Thus, $\rel$ is a simulation.
\end{proof}
